# Supplementary material for: Clingo goes Linear Constraints over Reals and Integers
Source: arXiv:1707.04053 source file (2017-07-13)
Supplement: Supplementary file 1 [file appendix.tex]

\newpage
\section*{Appendix}
\noindent\textit{Proposition~\ref{thm:settings}} \\
  \noindent
  Let $P$ be an lc-program over $\mathcal{A}\cup\mathcal{L}$
  and $P'$   an lc-program over $\mathcal{A}\cup\mathcal{L}'$
  such that $P=P'$.
  \begin{enumerate}
  \item \label{th:dsr} % X_d subseteq X_r
    If
    \(
    \mathcal{L}=\mathcal{L}\cap\head{P}
    \),
    then
    \(
    \smsetlc{P}\subseteq\smset{P}
    \)
  \item \label{th:rsen} % X_r subseteq X_en
    If
    \(
    \mathcal{L}=\mathcal{L}^\rightarrow\setminus\head{P}
    \),
    then
    \(
    \smset{P}\subseteq\smsetlc{P}
    \)
  \item \label{th:ssn} % X_s subseteq X_n
    If
    \(
    \mathcal{L}'=\mathcal{L}'^\rightarrow
    \),
    then
    \(
    \smsetlc{P}\subseteq\smsetlc{P'}
    \)
  \end{enumerate}
  
\noindent\textit{Proof of Proposition~\ref{thm:settings}.\ref{th:dsr}}  
    \begin{itemize}
     \item The lc-atoms of $P$ are of type defined only, thus 
        \(
        \mathcal{L}=
        \mathcal{L}\cap\head{P}
        \). 
     \item If 
        \(
        \code{a}\in\mathcal{L}^\leftrightarrow
        \), then 
        $\PS{P}{\mathcal{S}}$ contains either 
        `\code{:- not a.}' or `\code{:- a.}' 
        regarding to 
        $\code{a}\in\mathcal{S}$ or 
        $\code{a}\not\in\mathcal{S}$, respectively.  
     \item On the other hand, if 
        \(
        \code{a}\in\mathcal{L}^\rightarrow
        \) then 
        $\PS{P}{\mathcal{S}}$ may contain just the latter one. 
     \item Due to the fact that adding an integrity rule to a program 
        can just remove regular stable models, 
        we obtain 
        \(
        \smsetlc{P}\subseteq\smset{P}
        \). 
        $\hfill\square$
    \end{itemize}
  
\noindent\textit{Proof of Proposition~\ref{thm:settings}.\ref{th:rsen}}
    \begin{itemize}
     \item The lc-atoms of $P$ are of type 
        \lcatype{external}{non-strict} only, thus 
        \(
        \mathcal{L}=
        \mathcal{L}^\rightarrow\setminus\head{P}
        \). 
     \item Note that in this case 
        $\emptyset\subseteq\mathcal{L}$ 
        is always an lc-solution, 
        since (i) and (ii) are trivially satisfied. 
     \item Then we obtain 
        $P=\PS{P}{\emptyset}$ 
        and thus 
        \(
        \smset{P}=
        \smset{\PS{P}{\emptyset}}
        \). 
     \item If $\mathcal{S}\neq\emptyset$ 
        then $\PS{P}{\mathcal{S}}$ may includes choice rules 
        containing lc-atoms, and thus we probably obtain an
        lc-stable model $X\not\in\smset{P}$. 
     \item Finally, 
        \(
        \smset{P}\subseteq\smsetlc{P}
        \) 
        holds.
        $\hfill\square$
    \end{itemize}

\noindent\textit{Proof of Proposition~\ref{thm:settings}.\ref{th:ssn}}   
    \begin{itemize}
     \item If $\mathcal{L}=\mathcal{L}^\rightarrow$, 
        then $\smsetlc{P}=\smsetlc{P'}$ holds trivially.
     \item Due to this observation it is sufficient to assume 
        \(
        \mathcal{L}=
        \mathcal{L}^\leftrightarrow
        \). 
     \item The lc-atoms of $P$ are of type 
        strict only and 
        the lc-atoms of $P'$ are of type
        non-strict only, thus  
        \(
        \mathcal{L}=
        \mathcal{L}^\leftrightarrow
        \) 
        and
        \(
        \mathcal{L}'=
        \mathcal{L}'^\rightarrow
        \) respectively.  
     \item First, note that 
        \(
        \{\mathcal{S}\mid\mathcal{S}\subseteq\mathcal{L}\text{ lc-solution}\}\subseteq
        \{\mathcal{S}\mid\mathcal{S}\subseteq\mathcal{L}'\text{ lc-solution}\}
        \), 
        since elements of the first set need to satisfy (i) and (ii), 
        where elements of the latter just need to satisfy (i). 
     \item This observation leads to 
        \(
        \smsetlc{P}\subseteq\smsetlc{P'}
        \) 
        regarding to $\{\mathcal{S}\mid\mathcal{S}\subseteq\mathcal{L}\text{ lc-solution}\}$, 
        since \PS{P}{\mathcal{S}} with $\code{a}\in\mathcal{S}$ 
        contains either `\code{a.}' or `\code{:- not a.}' for 
        $\code{a}\in\mathcal{L}\setminus\head{P}$ or 
        $\code{a}\in\mathcal{L}\cap\head{P}$, respectively. 
     \item Whereas \PS{P'}{\mathcal{S}} contains just `\code{\{a\}.}' 
        for $\code{a}\in\mathcal{L}'\setminus\head{P}$. 
     \item Obviously, the latter leads to more stable models, 
        due to choice rules and the absence of integrity rules.
     \item Note that we can omit observations for 
        $\code{a}\not\in\mathcal{S}$, 
        since this case adds the same integrity for 
        both \PS{P}{\mathcal{S}} and \PS{P'}{\mathcal{S}}. 
     \item If we now consider 
        \(
        \mathcal{S}\in\{\mathcal{S}\mid\mathcal{S}\subseteq\mathcal{L}'\text{ lc-solution}\}\setminus
        \{\mathcal{S}\mid\mathcal{S}\subseteq\mathcal{L}\text{ lc-solution}\}
        \), 
        then we note that this cannot remove lc-stable models of 
        $\smsetlc{P'}$ that we already got from 
        \(
        \{\mathcal{S}\mid\mathcal{S}\subseteq\mathcal{L}\text{ lc-solution}\}
        \), 
        it can only be the case that we obtain additional stable models. 
     \item Finally, we get 
        \(
        \smsetlc{P}\subseteq\smsetlc{P'}
        \), 
        regarding their respective signature. 
        $\hfill\square$
    \end{itemize}

\noindent\textit{Proposition~\ref{thm:settings2}} \\
\noindent    
There exist lc-programs $P$ over $\mathcal{A}\cup\mathcal{L}$ with
\(
\mathcal{L}=\mathcal{L}^\leftrightarrow\setminus\head{P}
\),
so that
\(
\smset{P}\not\subseteq\smsetlc{P}
\)
or
\(
\smsetlc{P}\not\subseteq\smset{P}
\).\\[2mm]
\noindent\textit{Proof of Proposition~\ref{thm:settings2}}
    \begin{itemize}
     \item The lc-atoms of $P$ are of type 
        \lcatype{external}{strict} only, thus 
        \(
        \mathcal{L}=
        \mathcal{L}^\leftrightarrow\setminus\head{P}
        \). 
     \item The proof based on the property of lc-theory 
        that the theory consists contradicting elements (e.g. inverse elements).   
     \item First, we show 
        \(
        \smset{P}\not\subseteq\smsetlc{P}
        \). 
     \item Let $P=\{$\lstinline@ :- @$\code{a}$\lstinline@.  :- @$\overline{\code{a}}$\lstinline@.@$\}$, 
        where          $\overline{\code{a}}\in\mathcal{L}$ 
        represents the inverse of $\code{a}\in\mathcal{L}$. 
     \item Obviously, $\smset{P}=\{\emptyset\}$. 
     \item On the other hand, 
        $\mathcal{S}=\{\code{a}\}$ and 
        $\mathcal{S}'=\{\overline{\code{a}}\}$ 
        are the only lc-solutions regarding to strict semantics. 
     \item Thus, 
        $\PS{P}{\mathcal{S}}=P\cup\{\code{a.}\}$ and 
        $\PS{P}{\mathcal{S}'}=P\cup\{\overline{\code{a}}.\}$, 
        which is contradicting to 
        `\lstinline@ :- @$\code{a.}$' and 
        `\lstinline@:- @$\overline{\code{a}}.$', respectively. 
     \item We get 
        $\smsetlc{P}=\emptyset$ and thus 
        \(
        \smset{P}\not\subseteq\smsetlc{P}
        \). 
     \item Let now $P=\{$\lstinline@:- not @$\code{a.}\}$ 
        with $\smset{P}=\emptyset$. 
     \item Note that $\mathcal{S}=\{\code{a}\}$ is a lc-solutions. 
     \item We obtain 
        \(
        \PS{P}{\mathcal{S}}=
        P\cup\{\code{a.}\}
        \) 
        with 
        \(
        \smset{\PS{P}{\mathcal{S}}}=
        \{\{\code{a}\}\}
        \). 
     \item Thus 
        \(
        \smsetlc{P}\not\subseteq\smset{P}
        \)  
        holds. 
        $\hfill\square$
    \end{itemize}

%%% Local Variables:
%%% mode: latex
%%% TeX-master: "paper"
%%% End:
